# Supplementary material for: DHEN: A Deep and Hierarchical Ensemble Network for Large-Scale Click-Through Rate Prediction
Source: arXiv:2203.11014 source file (2022-03-11)
Supplement: Supplementary file 1 [file 8-appendix.tex]

\section*{Appendix}

In addition, authors can provide an optional two (2) page supplement at the end of their submitted paper (it needs to be in the same PDF file and start at page 10) focused on reproducibility (see reproducibility section for more details). After the submission deadline, the set of authors cannot be changed.
